# Supplementary material for: Waveforms for xG Non-stationary Channels
Source: arXiv:2301.00454 source file (2023-08-30)
Supplement: Supplementary file 2 [file appendix_AE.tex]

\appendices
\label{appendix:AE}
\section{Derivation of interference-free communication}
\begin{align}
     &r(u,t) {=} \int \sum\nolimits_{u'} h_{u,u'}(t,\tau) x_{u'}(t-\tau) d\tau + v_{u}(t) \nonumber \\
     &{=} \iint k_H(u,t;u',t') x(u',t')~du'~dt' + v(u{,}t) \nonumber \\
     &{=} \iint \sum\nolimits_{n{=1}}^\infty  \sigma_n \psi_n(u,t) \phi_n(u',t') \sum_{n'{=}1}^\infty x_{n'} \phi_{n'}^*(u{,}t)~du'~dt'\nonumber \\
     &{+} v(u,t)\nonumber  \\
    & {=} \iint \sum\nolimits_{n{=1}}^\infty  \sigma_n x_n \psi_n(u,t) |\phi_n(u',t')|^2 \nonumber \\
     &{+}\sum_{n'{\neq}n}^\infty \sigma_n x_{n'} \phi_n(u',t')\phi_{n'}^*(u{,}t)~du'~dt' + v(u{,}t) \nonumber \\
    & {=} \sum\nolimits_{n{=1}}^\infty  \sigma_n x_n \psi_n(u,t) \delta_{nn}
     {+}\sum_{n'{\neq}n}^\infty \sigma_n x_{n'}\delta_{nn'} +  v(u{,}t)  \nonumber \\
    & {=}\sum\nolimits_{n{=1}}^\infty s_n \psi_n(u,t) +  v(u{,}t)\nonumber  \\
    & {=} s(u{,}t) + v(u{,}t)
\end{align}

\section{Proof of Theorem 1: Correctness of AE for HOGMT}
% \textbf{Proof of Correctness (AE extracts the TED (KLT eigenfunctions)):}
Consider the AE loss function $\mathcal{L}{=}\mathcal{J}{+}\Omega$, where $\mathcal{J}{=}\|\textbf{x}-\hat{\textbf{x}}\|^2$ ($\textbf{x}$ represents each column of the hankel matrix $\textbf{U}$ which is used to train the AE) and $\Omega$ as defined below,
\begin{equation}
% \small
% \operatorname{L}_{KLT}(\Phi)=-\sum_{i=1}^{m} \phi_{i}^{\mathrm{T}} Q \phi_{i}+ \gamma \sum_{i=1}^{m}\left(\phi_{i}^{T} \phi_{i}-1\right)+ \beta \sum_{i=1}^{m} \sum_{j=1}^{i-1} \phi_{i}^{T} \phi_{j}+ \eta \sum_{i=1}^{m} \sum_{j=1}^{i-1}  \phi_{i}^{T} Q \phi_{j}
% \Omega(\boldsymbol{W}_{dec})= \lambda \left(\sum_{i{=}1}^{M}\left(w_{i}^{H} \phi_{i}-1\right)+ \sum_{i=1}^{M} \sum_{j=1}^{i-1} \phi_{i}^{H} \phi_{j}+ \sum_{i=1}^{M} \sum_{j=1}^{i-1}  \phi_{i}^{H} \mathbf{R_{\mathbf{xx}}} \phi_{j} \right)
\Omega(\boldsymbol{W}_{dec})= \lambda \left([\boldsymbol{W}_{dec}^H\boldsymbol{W}_{dec}-\boldsymbol{I}] + \boldsymbol{W}_{dec}^H\mathbf{R_{\mathbf{xx}}}\boldsymbol{W}_{dec}\right)
\label{eq:KLT}
% \vspace{-10pt}
\end{equation}
$\mathbf{R_{\mathbf{xx}}}$ is the input correlation matrix, and  $\lambda{>}0$ is a constant used to penalize the deviation from the KLT eigen bases. The first term ensures that the basis vectors are orthonormal and the final term ensures that the transformed signal components are uncorrelated.

\textbf{Proof:} 
We first observe that finding the eigenfunctions in KLT decomposition and reconstruction is equivalent to solving the following objective function: $\min _{\mathbf{\Phi}}\left\|\mathrm{U}-\mathrm{\Phi\Phi}^{T} \mathrm{U}\right\|_{F}^{2} \text { s.t. } \mathrm{\Phi}^{T} \mathrm{\Phi}=\mathrm{I}$, where $U$ is the Hankel matrix.
Given the linear AE is trained by sequentially feeding in each column of $U$ (denoted as $x$), the encoder and decoder is given by $y=W_{enc}x$ and $\hat{x}=W_{dec}y$. Since the cost function $\mathcal{J}$ is the total squared difference between output and input, then training the autoencoder on the input hankel matrix $\textbf{U}$ solves the following: $\min_{\boldsymbol{\Phi}}\left\|\mathrm{U}-\mathrm{W}_{dec} \mathrm{W}_{enc} \mathrm{U}\right\|_{F}^{2}{+}\Omega_{TED}(\boldsymbol{\Phi})$. 
In \cite{NN_PCA} it is shown that when setting the gradients to zero, $W_{enc}$ is the left Moore-Penrose pseudoinverse of $\mathrm{W}_{dec}$): $\mathrm{W}_{enc}=\mathrm{W}_{dec}^{\dagger}=\left(\mathrm{W}_{dec}^{H} \mathrm{~W}_{dec}\right)^{-1} \mathrm{~W}_{dec}^{H}$ and hence the loss function becomes $\min_{\boldsymbol{\Phi}}\left\|\mathrm{U}-\mathrm{W}_{dec} \mathrm{W}_{dec}^{\dagger} \mathrm{U}\right\|_{F}^{2}{+}\Omega_{TED}(\boldsymbol{\Phi})$. The regularization function $\Omega_{TED}(\boldsymbol{\Phi})$ ensures that the weights are orthonormal, i.e., $\mathrm{W}_{dec} \mathrm{W}_{dec}^{H}=\textbf{I}$, and therefore implies that $\mathrm{W}_{enc}{=}\mathrm{W}_{dec}^{H}$. Then minimizing the loss function of the AE is equivalent to minimizing the objective in KLT since the KLT optimization and AE loss functions are equivalent and the eigen decomposition is a unique representation.
Therefore, we have that $\mathrm{W}_{dec}{=}\mathrm{W}_{enc}^H$ is the same as $\Phi$.
This can be extended to show that a nonlinear AE extracts the nonlinear kernel-KLT eigenfunctions.
% Meanwhile, the KLT coefficents are uncorrelated, which means in autoencoder, the features should also be uncorrelated
% \begin{equation}
%     corr(\sigma_i, \sigma_j) = 0,~\text{for}~i \neq j.
% \end{equation}

\textbf{a) Extension to Deep Autoencoders:}
Let $W_1,{\ldots},W_d$ be the weight matrices corresponding to the $d$ layers at the encoder. Then we calculate $W_{enc}$ or $W_{dec}$ from the trained weights after training as, $W_{enc}=W_1W_2{\ldots}W_d=W_{dec}^H$. Then the proof above holds \cite{ghojogh2019unsupervised}.   

\textbf{b) Extension to Nonlinear Deep Autoencoders:}
Let $W_1,{\ldots},W_d$ be the nonlinear functions corresponding to the $d$ layers at the encoder. Then we calculate $W_{enc}$ or $W_{dec}$ from the trained weights and biases (or from the functions they describe) after training as, $W_{enc}(x)=W_d({\ldots}(W_2(W_1(x)){\ldots})$. Then $W_{dec}$ learns a kernel or non-linear eigen transformation \cite{ghojogh2019unsupervised}.
