# Supplementary material for: Waveforms for xG Non-stationary Channels
Source: arXiv:2301.00454 source file (2023-08-30)
Supplement: Supplementary file 3 [file appendix_old.tex]

\appendices
\label{appendix:precoding}

% \begin{multicols}{2}
% [
% \begin{center}
% \large{\textbf{Proofs and Supplementary Material:\\ Unified Characterization and Precoding for Non-Stationary Channels}}\\

% \vspace{5pt}
% \normalsize
% Zhibin Zou\textsuperscript{\textbf{*}}, Maqsood Careem\textsuperscript{\textbf{*}}, Aveek Dutta\textsuperscript{\textbf{*}} \& \\
% Ngwe Thawdar\textsuperscript{\textbf{**}} \\

% \vspace{5pt}
% \small
% \textsuperscript{\textbf{*}}Department of Electrical and Computer Engineering,\\ 
% University at Albany SUNY, Albany, NY 12222 USA\\
% \textsuperscript{\textbf{**}}US Air Force Research Laboratory,\\
% Rome, NY, USA
% \end{center}

% \normalsize

\noindent
\textbf{Instructions:}
Equations (1)--(34) refer to the equations from the main manuscript (``Unified Characterization and Precoding for Non-Stationary Channels" accepted for publication at IEEE ICC 2022). This document provides the supplementary material including a comprehensive related work, the complete proofs and extended evaluation results to support the main manuscript.  
% Equations \eqref{eq:H_delay_Doppler}--\eqref{eq:xut} and the references [1]--[23] refer to the equations and references from the main manuscript (``Unified Characterization and Precoding for Non-Stationary Channels" accepted for publication at IEEE ICC 2022), respectively. This document provides the supplementary material including a comprehensive related work, the complete proofs and extended evaluation results to support the main manuscript.  

% \noindent
% % ]
% \end{multicols}


\input{related_NLP}

\begin{comment}
\section{Proof of Proposition 1:}
\label{App:pro_1}
\begin{proof}
\note{May not use this result}
From \eqref{eq:atomic}, if the transmit signal is $s(t',f')$, the received signal $r(t',f')$ is 
\begin{align}
\label{eq:rec_r}
   & r(t',f') = \iiiint \mathcal{H}(t, f ; \tau, \nu) \mathbf{S}_{t,f}^{\tau,\nu}(t',f') ~dt ~df ~d\tau ~dv \nonumber \\ 
   & = \iiiint \mathcal{H}(t, f ; \tau, \nu) \nonumber \\
   & \times s(t'-t,f'-f) e^{-j2\pi (\nu t' - \tau (f'+f))} ~dt ~df ~d\tau ~dv \nonumber \\ 
   & = \iint \left\{ \iint \mathcal{H}(t, f ; \tau, \nu)e^{-j2\pi (\nu t' - \tau (f'+f))} ~d\tau ~dv \right\} \nonumber \\
   & \times s(t'-t,f'-f) ~dt ~df  
\end{align}

From \eqref{eq:compute_H}, we have
\begin{align}
\label{eq:simplify_H}
&\iint \mathcal{H}(t, f ; \tau, \nu)e^{-j2\pi (\nu t' - \tau (f'+f))} ~d\tau ~dv \nonumber \\
& = \iiiint L_{\mathbf{H}}\left(t^{\prime}, f^{\prime}\right) L_{\mathbf{G}}^{*}\left(t^{\prime}-t, f^{\prime}-f\right) \nonumber \\
& \times \mathrm{e}^{-2 \times j 2 \pi\left(\nu t^{\prime}-\tau (f^{\prime} + f )\right)} \mathrm{d} t^{\prime} \mathrm{d} f^{\prime} \mathrm{d} \tau \mathrm{d} \nu \nonumber \\
& = L_{\mathbf{H}}\left(- t^{\prime}, - f^{\prime} + f \right) L_{\mathbf{G}}^{*}\left( - t^{\prime}-t, - f^{\prime} \right)
\end{align}
where first transfer $(t',f'+f)$ to $(\nu,\tau)$ and then transfer $(\nu,\tau)$ to $(-t', -(f'+f))$. Substitute \eqref{eq:simplify_H} in \eqref{eq:rec_r} 
\begin{align}
   & r(t',f') \nonumber \\ 
   & = \iint  L_{\mathbf{H}}\left(- t^{\prime}, - f^{\prime} + f\right) L_{\mathbf{G}}^{*}\left( - t^{\prime}-t, - f^{\prime}\right) \nonumber \\
   & \times s(t'-t,f'-f) ~dt ~df  
\end{align}

Swipe $(t, f)$ and $(t',f')$, finally,
\begin{align}
   & r(t,f) = \iint  h(t,f;t',f') s(t-t',f-f') ~dt' ~df'  
\end{align}
where $h(t,f;t',f') = L_{\mathbf{H}} (-t,-f + f') L_{\mathbf{G}}^*(-t-t', -f)$.
\end{proof}
\end{comment}



\section{Proofs on Unified Characterization}
\label{app:characterization}

\subsection{Proof of Lemma 1: Generalized Mercer's Theorem}
\label{App:gmt}

\begin{proof}
Consider a 2-dimensional process $K(t,t') \in L^2(Y \times X)$, where $Y(t)$ and $X(t')$ are square-integrable zero-mean random processes with covariance function $K_{Y}$ and $K_{X}$, respecly. 
% 
The projection of $K(t, t')$ onto $X(t')$ is obtained as in \eqref{eq:projection},
\begin{align}
\label{eq:projection}
    & C(t) = \int K(t, t') X(t') ~dt'
\end{align}

Using \textit{Karhunen–Loève Transform} (KLT), $X(t')$ and $C(t)$ are both decomposed as in \eqref{eq:X_t} and \eqref{eq:C_t}, 
\begin{align}
    &X(t') = \sum_{i = 1}^{\infty} x_{i} \phi_{i}(t') \label{eq:X_t}\\
    &C(t) = \sum_{j = 1}^{\infty} c_{j} \psi_{j}(t) \label{eq:C_t}
\end{align}
where $x_i$ and $c_j$ are both random variables with $\mathbb{E}\{x_i x_{i'}\} {=} \lambda_{x_i} \delta_{ii'}$ and $\mathbb{E}\{c_j c_{j'}\} {=} \lambda_{c_j} \delta_{jj'}$.  $\{\lambda_{x_i}\}$, $\{\lambda_{x_j}\}$ $\{\phi_i(t')\}$ and $\{\psi_j(t)\}$ are eigenvalues and eigenfuncions, respectively.
% of $T_{K_{X}}$ and $T_{K_{C}}$, respectively. 
% 

Let us denote $n{=}i{=}j$ and $\sigma_n {=} \frac{c_n}{x_n}$, and assume that $K(t,t')$ can be expressed as in \eqref{eq:thm_K_t},
\begin{align}
\label{eq:thm_K_t}
    K(t,t') = \sum_n^\infty \sigma_n \psi_{n}(t) \phi_{n}(t')
\end{align}
We show that \eqref{eq:thm_K_t} is a correct representation of $K(t,t')$ by proving \eqref{eq:projection} holds under this definition. 
We observe that by substituting \eqref{eq:X_t} and \eqref{eq:thm_K_t} into the right hand side of \eqref{eq:projection} we have that,
\begin{align}
    & \int K(t, t') X(t') ~dt' \nonumber \\
    & = \int \sum_n^\infty \sigma_n \psi_{n}(t) \phi_{n}(t') \sum_{n}^{\infty} x_{n} \phi_{n}(t') ~dt' \nonumber \\
    & = \int \sum_n^\infty \sigma_n x_n \psi_n(t) |\phi_n(t')|^2 \nonumber\\
    & + \sum_{n'\neq n}^ \infty \sigma_{n} x_{n'} \psi_{n}(t) \phi_{n}(t') \phi_{n'}^*(t') ~d t' \nonumber \\
    & = \sum_n^\infty c_n \psi_n(t) = C(t)
\end{align}
which is equal to the left hand side of \eqref{eq:projection}. 
Therefore, \eqref{eq:thm_K_t} is a correct representation of $K(t,t')$.

\begin{comment}
Substitute the left side of \eqref{eq:thm1_1} by \eqref{eq:thm1_2}, we have 
\begin{equation}
    \sum_{j = 1}^{\infty} \mu_{j} \psi_{j}(t) = \sum_{i = 1}^{\infty} z_i c_i(t)
\end{equation}

Notice $i$ and $j$ have the same range. Denote $n = i = j$ and $\sigma_n = \mu_n / z_n$, we have
\begin{align}
    &\sigma_n \psi_{n}(t) =  c_n(t) \nonumber \\ 
    & = \int K(t, t') \phi_{n}(t') ~dt'
\end{align}

Thus $K(t, t')$ can be decomposed
\begin{align}
    K(t, t') = \sum_{n=1}^{\infty} \sigma_n \psi_n(t) \phi_n(t') 
\end{align}
where $E\{\sigma_n \sigma_n'\} = \lambda_n \delta_{nn'}$. $\lambda_n$ is eigenvalue. $\psi_n(t)$ and $\phi_n(t')$ are both eigenfunctions.
\end{comment}

\begin{comment}
Consider a P-dimensional process $K \in L^P(X_1 \times X_2\times \cdots \times X_P)$.

For a square-integrable zero-mean random process process $X_i, i\in \{1, 2, \cdots, P\}$, with covariance function $K_{X_i}$ Karhunen–Loève theorem gives 

\begin{equation}
    X_i = \sum_{n}^{\infty} \sigma_{n}^{(i)} \phi_{n}^{(i)}(t_i)
\end{equation}
where $E\{\sigma_n^{(i)} \sigma_n'^{(i)}\} = \lambda_n^{(i)} \delta_{nn'}$. $\lambda_n^{(i)}$ and $\phi_n^{(i)}(t_i)$ are eigenvalue and eigenfuncion of $T_{K_{X_i}}$, respectively. 
\end{comment}
\end{proof}


\subsection{Proof of Theorem 1: High Order Generalized Mercer's Theorem (HOGMT}
\label{app:hogmt}

\begin{proof}
Given a 2-D process $X(\gamma_1, \gamma_2)$, the eigen-decomposition using Lemma \ref{lemma:GMT} is given by,
\begin{equation}
\label{eq:thm1_1}
    X(\gamma_1, \gamma_2) = \sum_{n}^{\infty} x_{n} e_n(\gamma_1) s_n(\gamma_2)
\end{equation}

Letting $\psi_n(\gamma_1,\gamma_2) {=} e_n(\gamma_1) s_n(\gamma_2)$, and substituting it in \eqref{eq:thm1_1} we have that,

\begin{equation}
\label{eq:2d_klt}
    X(\gamma_1, \gamma_2) = \sum_{n}^{\infty} x_{n} \phi_n(\gamma_1,\gamma_2)
\end{equation}
where $\phi_n(\gamma_1,\gamma_2)$ are 2-D eigenfunctions with the property \eqref{eq:prop1}.
\begin{equation}
\label{eq:prop1}
\iint \phi_n(\gamma_1,\gamma_2) \phi_{n'}(\gamma_1,\gamma_2) ~d\gamma_1 ~d\gamma_2 = \delta_{nn'} 
\end{equation}

We observe that \eqref{eq:2d_klt} is the 2-D form of KLT. With iterations of the above steps, we obtain \textit{Higher-Order KLT} for $X(\gamma_1,\cdots,\gamma_Q)$ and $C(\zeta_1,\cdots,\zeta_P)$ as given by,
\begin{align}
   & X(\gamma_1,\cdots,\gamma_Q) = \sum_{n}^{\infty} x_{n} \phi_n(\gamma_1,\cdots,\gamma_Q) \\
   & C(\zeta_1,\cdots,\zeta_P) = \sum_{n}^{\infty} c_{n} \psi_n(\zeta_1,\cdots,\zeta_P)
\end{align}
where $C(\zeta_1,\cdots,\zeta_P)$ is the projection of $X(\gamma_1,\cdots,\gamma_Q)$ onto $K(\zeta_1,\cdots,\zeta_P; \gamma_1,\cdots, \gamma_Q)$.

Then following similar steps as in Appendix~\ref{App:gmt} we get \eqref{eq:col}. 
\begin{align}
\label{eq:col}
& K(\zeta_1,\cdots,\zeta_P; \gamma_1,\cdots, \gamma_Q) \nonumber \\
& = \sum_{n}^ \infty \sigma_n \psi_n(\zeta_1,\cdots,\zeta_P) \phi_n(\gamma_1,\cdots, \gamma_Q)
\end{align}
\end{proof}




\section{Proofs on Eigenfunction based Precoding}
\label{app:precoding}

\subsection{Proof of Lemma 2}
\label{app:lem1}

\begin{proof}
Using 2-D KLT as in \eqref{eq:GMT_2D}, $x(u,t)$ is expressed as,
\begin{equation}
    x(u,t) = \sum_{n}^ \infty x_n \phi_n(u,t)
\end{equation}
where $x_n$ is a random variable with $E\{x_n x_{n'}\}{=} \lambda_n \sigma_{nn'} $ and $\phi_n(u,t)$ is a 2-D eigenfunction. 

\begin{comment}
\begin{align}
    & E\{|x(u,t)|^2\} = E\{|\sum_{n}^ \infty x_n \phi_n(u,t)|^2\} \nonumber\\
    & = \sum_{n}^ \infty E\{|x_n|^2\} E\{|\phi_n(u,t)|^2\} \nonumber \\
    & = \sum_{n}^ \infty \frac{\lambda_n}{T}\iint_{T}|\phi_n(u,t)|^2 ~du ~dt  \nonumber \\
    & = \sum_{n}^ \infty \frac{\lambda_n}{T} 
\end{align}
where $T$ is the time interval. Then minimizing $E\{|x(t)|^2\}$ converts to minimizing $\sum_j^ \infty \lambda_j$.
\end{comment}

Then the projection of $k_H(u,t;u',t')$ onto $\phi_n(u',t')$ is denoted by $ c_n(u,t)$ and is given by,
\begin{equation}
    c_n(u,t) =  \iint k_H(u,t;u',t') \phi_n(u',t') ~du' ~dt'
\end{equation}

Using the above, \eqref{eq:obj} is expressed as,
\begin{align}
\label{eq:obj_trans}
     & ||s(u,t) - Hx(u,t)||^2 = ||s(u,t) - \sum_n^ \infty x_n c_n(u,t)||^2
\end{align}

Let $\epsilon (x) {=} ||s(u,t) - \sum_n^ \infty x_n \phi_n(u,t)||^2$. Then its expansion is given by,
\begin{align}
\label{eq:ep}
     & \epsilon (x) = \langle s(u,t),s(u,t) \rangle - 2\sum_n ^ \infty  x_n \langle c_n(u,t),s(u,t) \rangle \\
     & + \sum_n^ \infty x_n^2 \langle c_n(u,t), c_n(u,t) \rangle \nonumber + \sum_n^ \infty \sum_{n' \neq n}^ \infty x_n x_{n'}  \langle c_n(u,t), c_{n'}(u,t) \rangle
\end{align}

Then the solution to achieve minimal $\epsilon(x)$ is obtained by solving for $\pdv{\epsilon(x)}{x_n} = 0$ as in \eqref{eq:solution}.
\begin{align}
\label{eq:solution}
    x_n^{opt} & {=}  \frac{\langle s(u,t), c_n(u,t) \rangle + \sum_{n'\neq n}^ \infty x_{n'} \langle c_{n'}(u,t), c_n(u,t) \rangle }{\langle c_n(u,t), c_n(u,t) \rangle}
\end{align}
where $\langle a(u,t), b(u,t) \rangle {=} \iint a(u,t) b^*(u,t) ~du ~dt$ denotes the inner product. 
% 
Let $\langle c_{n'}(u,t), c_n(u,t) \rangle = 0$, i.e., the projections $\{ c_n(u,t)\}_n$ are orthogonal basis. Then we have a closed form expression for $x^{opt}$ as in \eqref{eq:x_opt}.
\begin{align}
\label{eq:x_opt}
    x_n^{opt} & {=}  \frac{\langle s(u,t), c_n(u,t) \rangle}{\langle c_n(u,t), c_n(u,t) \rangle}
\end{align}

Substitute \eqref{eq:x_opt} in \eqref{eq:ep}, it is straightforward to show that $\epsilon(x){=} 0$.
\end{proof}



\subsection{Proof of Theorem 2: Eigenfunction Precoding}
\label{app:thm_2}
\begin{proof}
The 4-D kernel $k_H(u,t;u',t')$ is decomposed into two separate sets of eigenfunction $\{\phi_n(u',t')\}$ and $\{\psi_n(u, t) \}$ using Theorem 1 as in \eqref{eq:thm2_decomp}. By transmitting the conjugate of the eigenfunctions, $\phi_n(u',t')$ through the channel $H$, we have that,  
\begin{align}
   & H \phi_n^*(u',t') = \iint k_H(u,t;u',t') \phi_n^*(u',t') ~du' ~d t' \nonumber \\ 
   & {=} \iint \sum_{n}^ \infty \{\sigma_n \psi_n(u,t) \phi_n(u',t')\} \phi_n^*(u',t') ~d t' ~d f' \nonumber \\ 
   & {=} \iint \sigma_n \psi_n(u,t) |\phi_n(u',t')|^2 \nonumber\\
   & + \sum_{n'\neq n}^ \infty \sigma_{n'} \psi_{n'}(u,t) \phi_{n'}(u',t')\ \phi_n^*(u',t') ~du' ~d t' \nonumber \\
   & {=} \sigma_n \psi_n(u,t)
\end{align}
where $\psi_n(u,t)$ is also a 2-D eigenfunction with the orthogonal property as in \eqref{eq:thm2_decomp_pty}. 

From Lemma~\ref{lemma:bestprojection}, if the set of projections, $\{c_n(u,t)\}$ is the set of eigenfunctions, $\{\psi_n(u,t)\}$, which has the above orthogonal property, we achieve the optimal solution as in \eqref{eq:x_opt}. Therefore, let $x(u,t)$ be the linear combination of $\{\phi_n^*(u,t)\}$ with coefficients $\{x_n\}$ as in \eqref{eq:construct},

\begin{equation}
\label{eq:construct}
    x(u,t) = \sum_n^ \infty x_n \phi_n^*(u,t) 
\end{equation}


Then \eqref{eq:obj_trans} is rewritten as in \eqref{eq:obj_trans2},
\begin{align}
\label{eq:obj_trans2}
     & ||s(u,t) - Hx(u,t)||^2 = ||s(u,t) - \sum_n^ \infty x_n \sigma_n \psi(u,t)||^2
\end{align}
   
Therefore, optimal $x_n$ in \eqref{eq:x_opt} is obtained as in \eqref{eq:opt},

\begin{equation}
\label{eq:opt}
    x_n^{opt} = \frac{\langle s(u,t), \psi_n(u,t) \rangle}{\sigma_n} 
\end{equation}

Substituting \eqref{eq:opt} in \eqref{eq:construct}, the transmit signal is given by \eqref{eq:x_opt2},
\begin{equation}
\label{eq:x_opt2}
    x(u,t) = \sum_n^ \infty \frac{\langle s(u,t), \psi_n(u,t) \rangle}{\sigma_n} \phi_n^*(u,t). 
\end{equation}
\end{proof}

\subsection{Proof of Corollary 1}
\label{app:EP_space}
\begin{proof}
First we substitute the 4-D kernel $k_H(u,t;u',t')$ with the 2-D kernel $k_H(u,u')$ in Theorem 2 which is then decomposed by the 2-D HOGMT. Then following similar steps as in Appendix~\ref{app:thm_2} it is straightforward to show \eqref{eq:xut}.
\end{proof}

\section{Results on Interference}
\label{App:results_interference}
\begin{figure}[h]
  \centering
  \includegraphics[width=1\linewidth]{figures/hst_1_10_50_100.pdf}
  \caption{Kernel $k_H(u,t;u',t')$ for $u {=} 1$ at a) $t {=} 1$, b) $t {=} 10 $, c) $t {=} 50$ and d) $t {=} 100$.}
%   \note{Include z label and same scale.}}
  \label{fig:hst_1_10_50_100}
\label{fig:hst_1_10_50_100}
\end{figure}
Figure~\ref{fig:hst_1_10_50_100} shows the channel response for user $u {=} 1$ at $t{=}1$, $t{=}10$, $t{=}50$ and $t{=}100$, where at each instance, the response for user $u {=} 1$ is not only affected by its own delay and other users' spatial interference, but also affected by other users' delayed symbols. 
% We call it space-time joint interference.  
This is the cause of joint space-time interference which necessitates joint precoding in the 2-dimensional space using eigenfunctions that are jointly orthogonal.


\begin{comment}
\section{Implementation Supplement}



For 4-D kernel tensor $\mathbf{K}{\in}\mathrm{C}^{N_u{\times}T{\times}N_u{\times}T}$ and 2-D symbol vectors $\mathbf{r}, \mathbf{x}{\in}\mathrm{C}^{N_u{\times}T} $, we have the I/O relation (noise-free)
\begin{align}
    \mathbf{r}[u,t] = \sum_{u'=1}^{N_u} \sum_{t'=1}^{T} \mathbf{K}[u,t;u',t'] \mathbf{x}[u',t']
\end{align}
where $[\cdot]$ denote the entry. $N_u$ and $T$ is the number of users and time instances, respectively. Through invertible mapping $f{:}u{\times}t{\to}m$, we have $\mathbf{K}{\in}\mathrm{C}^{N_uT{\times}N_uT}$ and $\mathbf{r}, \mathbf{x}{\in}\mathrm{C}^{N_uT{\times}1} $. The I/O relation becomes 

\begin{align}
    \mathbf{r}[m]= \sum_{m'=1}^{N_uT} \mathbf{K}[m;m'] \mathbf{x}[m']
\end{align}
which is matrix multiplication $\mathbf{r} {=} \mathbf{K}\mathbf{x}$. Split $\mathbf{r}$, $\mathbf{K}$ and $\mathbf{x}$ to real parts $\mathbf{R}$ and imaginary parts $\mathbf{I}$, respectively. We can construct new kernel matrix and symbols vectors $\mathbf{r'}{=} \begin{bmatrix}\mathbf{R_r}\\\mathbf{I_r}\end{bmatrix}$, $\mathbf{K'}{=}\begin{bmatrix}
\mathbf{R_K} & \mathbf{-I_K}\\
\mathbf{I_K} & \mathbf{R_K}
    \end{bmatrix}$ and $\mathbf{x'}{=}\begin{bmatrix}
\mathbf{R_x}\\
\mathbf{I_x}
    \end{bmatrix} $ with same I/O relation $\mathbf{r'} {=} \mathbf{K'}\mathbf{x'}$ due to linear relation
\begin{align}
     \begin{bmatrix}
\mathbf{R_r}\\
\mathbf{I_r}
    \end{bmatrix}  =  \begin{bmatrix}
\mathbf{R_K} & \mathbf{-I_K}\\
\mathbf{I_K} & \mathbf{R_K}
    \end{bmatrix} \times      
    \begin{bmatrix}
\mathbf{R_x}\\
\mathbf{I_x}
    \end{bmatrix} 
\end{align}

Thus the complex space converts to real space, with the size of kernel matrix and symbol vectors increases as $\mathbf{K'}{\in}\mathrm{C}^{2N_uT{\times}2N_uT}$ and $\mathbf{r'}, \mathbf{x'}{\in}\mathrm{C}^{2N_uT{\times}1}$, which means number of basis increased. For the real space I/O relation, $\mathbf{x'}$ can be obtained by HOGMT-precoding with $\mathbf{K'}$ and $\mathbf{s'}$ ($\mathbf{s'}$ can also be obtained by the same mapping, split and construction). 

Then combine real and imaginary parts $\mathbf{x} = \mathbf{R_x} + i\mathbf{I_x}$, and do inverse mapping  $g{:}m{\to}u{\times}t$, we get the final precoded signal vector $\mathbf{x}[u,t]$. The implementation data flow is shown as Figure~\ref{fig:Data_flow}.

\begin{figure*}[t]
    \centering
    \includegraphics[width=0.9\linewidth]{figures/Implementation.pdf}
    \caption{Data flow}
    \label{fig:Data_flow}
    \vspace{-10pt}
\end{figure*}

Figure~\ref{fig:Ber_space_multimod} and Figure~\ref{fig:Ber_space_time_multimode} show the BER performance of HOGMT based spatial precoding and space-time precoding with $\epsilon{=}10^{-3}$ for BPSK, QPSK, 16QAM and 64QAM modulation, respectively. 

\begin{figure}[t]
\begin{subfigure}{.24\textwidth}
  \centering
  \includegraphics[width=1\linewidth]{figures/Ber_space_multimod.pdf}
  \caption{BER of HOGMT based spatial precoding}
  \label{fig:Ber_space_multimod}
\end{subfigure}
\begin{subfigure}{.24\textwidth}
  \centering
  \includegraphics[width=1\linewidth]{figures/Ber_space_time_multimod.pdf}
  \caption{BER of HOGMT based spatio-temporal precoding }
  \label{fig:Ber_space_time_multimode}
\end{subfigure}
  \caption{BER of HOGMT based precoding with $\epsilon{=}10^{-3}$ for BPSK, QPSK, 16QAM and 64QAM}
  \vspace{-5pt}
\end{figure}

\end{comment}







\begin{comment}
\section{Proof of Theorem 1: Correctness of AE for KLT}
% \textbf{Proof of Correctness (AE extracts the TED (KLT eigenfunctions)):}
Consider the AE loss function $\mathcal{L}{=}\mathcal{J}{+}\Omega$, where $\mathcal{J}{=}\|\textbf{x}-\hat{\textbf{x}}\|^2$ ($\textbf{x}$ represents each column of the hankel matrix $\textbf{U}$ which is used to train the AE) and $\Omega$ as defined below,
\begin{equation}
% \small
% \operatorname{L}_{KLT}(\Phi)=-\sum_{i=1}^{m} \phi_{i}^{\mathrm{T}} Q \phi_{i}+ \gamma \sum_{i=1}^{m}\left(\phi_{i}^{T} \phi_{i}-1\right)+ \beta \sum_{i=1}^{m} \sum_{j=1}^{i-1} \phi_{i}^{T} \phi_{j}+ \eta \sum_{i=1}^{m} \sum_{j=1}^{i-1}  \phi_{i}^{T} Q \phi_{j}
% \Omega(\boldsymbol{W}_{dec})= \lambda \left(\sum_{i{=}1}^{M}\left(w_{i}^{H} \phi_{i}-1\right)+ \sum_{i=1}^{M} \sum_{j=1}^{i-1} \phi_{i}^{H} \phi_{j}+ \sum_{i=1}^{M} \sum_{j=1}^{i-1}  \phi_{i}^{H} \mathbf{R_{\mathbf{xx}}} \phi_{j} \right)
\Omega(\boldsymbol{W}_{dec})= \lambda \left([\boldsymbol{W}_{dec}^H\boldsymbol{W}_{dec}-\boldsymbol{I}] + \boldsymbol{W}_{dec}^H\mathbf{R_{\mathbf{xx}}}\boldsymbol{W}_{dec}\right)
\label{eq:KLT}
\vspace{-10pt}
\end{equation}
$\mathbf{R_{\mathbf{xx}}}$ is the input correlation matrix, and  $\lambda{>}0$ is a constant used to penalize the deviation from the KLT eigen bases. The first term ensures that the basis vectors are orthonormal and the final term ensures that the transformed signal components are uncorrelated.

\textbf{Proof:} 
We first observe that finding the eigenfunctions in KLT decomposition and reconstruction is equivalent to solving the following objective function: $\min _{\mathbf{\Phi}}\left\|\mathrm{U}-\mathrm{\Phi\Phi}^{T} \mathrm{U}\right\|_{F}^{2} \text { s.t. } \mathrm{\Phi}^{T} \mathrm{\Phi}=\mathrm{I}$, where $U$ is the Hankel matrix.
Given the linear AE is trained by sequentially feeding in each column of $U$ (denoted as $x$), the encoder and decoder is given by $y=W_{enc}x$ and $\hat{x}=W_{dec}y$. Since the cost function $\mathcal{J}$ is the total squared difference between output and input, then training the autoencoder on the input hankel matrix $\textbf{U}$ solves the following: $\min_{\boldsymbol{\Phi}}\left\|\mathrm{U}-\mathrm{W}_{dec} \mathrm{W}_{enc} \mathrm{U}\right\|_{F}^{2}{+}\Omega_{TED}(\boldsymbol{\Phi})$. 
In \cite{NN_PCA} it is shown that when setting the gradients to zero, $W_{enc}$ is the left Moore-Penrose pseudoinverse of $\mathrm{W}_{dec}$): $\mathrm{W}_{enc}=\mathrm{W}_{dec}^{\dagger}=\left(\mathrm{W}_{dec}^{H} \mathrm{~W}_{dec}\right)^{-1} \mathrm{~W}_{dec}^{H}$ and hence the loss function becomes $\min_{\boldsymbol{\Phi}}\left\|\mathrm{U}-\mathrm{W}_{dec} \mathrm{W}_{dec}^{\dagger} \mathrm{U}\right\|_{F}^{2}{+}\Omega_{TED}(\boldsymbol{\Phi})$. The regularization function $\Omega_{TED}(\boldsymbol{\Phi})$ ensures that the weights are orthonormal, i.e., $\mathrm{W}_{dec} \mathrm{W}_{dec}^{H}=\textbf{I}$, and therefore implies that $\mathrm{W}_{enc}{=}\mathrm{W}_{dec}^{H}$. Then minimizing the loss function of the AE is equivalent to minimizing the objective in KLT since the KLT optimization and AE loss functions are equivalent and the eigen decomposition is a unique representation.
Therefore, we have that $\mathrm{W}_{dec}{=}\mathrm{W}_{enc}^H$ is the same as $\Phi$.
This can be extended to show that a nonlinear AE extracts the nonlinear kernel-KLT eigenfunctions.
% Meanwhile, the KLT coefficents are uncorrelated, which means in autoencoder, the features should also be uncorrelated
% \begin{equation}
%     corr(\sigma_i, \sigma_j) = 0,~\text{for}~i \neq j.
% \end{equation}

\textbf{a) Extension to Deep Autoencoders:}
Let $W_1,{\ldots},W_d$ be the weight matrices corresponding to the $d$ layers at the encoder. Then we calculate $W_{enc}$ or $W_{dec}$ from the trained weights after training as, $W_{enc}=W_1W_2{\ldots}W_d=W_{dec}^H$. Then the proof above holds \cite{ghojogh2019unsupervised}.   

\textbf{b) Extension to Nonlinear Deep Autoencoders:}
Let $W_1,{\ldots},W_d$ be the nonlinear functions corresponding to the $d$ layers at the encoder. Then we calculate $W_{enc}$ or $W_{dec}$ from the trained weights and biases (or from the functions they describe) after training as, $W_{enc}(x)=W_d({\ldots}(W_2(W_1(x)){\ldots})$. Then $W_{dec}$ learns a kernel or non-linear eigen transformation \cite{ghojogh2019unsupervised}.   

\end{comment}

\begin{comment}
\section{Proof of Lemma~\ref{lemma:1}}
\label{app:lemma_1}

\section{Proof of Lemma~\ref{lemma:2}}
\label{app:lemma_2}
Let $\widetilde{X}=\sum_{n}^{N} x_{n} \phi_{n}$, $\Delta X=\sum_{n}^{N} x_{n} \Delta \phi_n$, and $H=\sum_{n}^{N} \sigma_{n} \phi_{n}$. We have
\begin{equation}
\begin{aligned}
& E[H(\tilde{X} + \Delta X)] \\
= &\int \sum_{n}^{N} \sigma_{n} \phi_{n} \cdot \sum_{m} x_{m}\left(\phi_{m}+\Delta \phi_{m}\right) d t \\
= & \sum_{n}^ \infty \int \sigma_{n} \phi_{n} x_{n}\left(\phi_{n}+\Delta \phi_{n}\right)+\sum_{m \neq n}^ \infty \sigma_{n} \phi_{n} x_{m}\left(\phi_{n}+\Delta \phi_{m}\right) dt\\
= &\sum_{n}^ \infty \int \sigma_{n} x_{n} \phi_{n} \phi_{n} d t+\sum_{m}^{N} \sigma_{n} x_{n} \phi_{n} \Delta \phi_{m} d t +\sum_{n' \neq n}^{N} \sigma_{n} x_{m} \phi_{n} \phi_{n'} d t\\
= &\sum_{n}^{N}\left[\sigma_{n} x_{n}+\sum_{m}^{N} \frac{\sigma_{n} x_{m}\left\langle\phi_{n}, \Delta \phi_{m}\right\rangle}{x_{n}} \cdot x_{n}\right]
\end{aligned}
\end{equation}

Let
\begin{equation}
\Delta \sigma_{n}=\frac{\sigma_{n} \sum_{m} x_{m} \langle \phi_{n}, \Delta \phi_{m}\rangle}{x_{n}}
\end{equation}

We have 

\begin{equation}
\begin{aligned}
E[H(\tilde{X} + \Delta X)]= & \sum_{n}^{N}\left[\sigma_{n}+\Delta \sigma_{n}\right] x_{n}=E[(H+\Delta H) \widetilde{X}]
\end{aligned}
\end{equation}

\section{Proof of Lemma~\ref{lemma:3}}
\label{app:lemma_3}

The received signal can be written as
\begin{equation}
Y = HX + W.    
\end{equation}

Let $E\{W^2\} = \sigma^2_W$. We have
\begin{equation}
\begin{aligned}
& E\{H X\} \\
=& \int \sum_{n}^{N} \sigma_{n} \phi_{n} \cdot \sum_{m}^{N} X_{m}(\langle \hat{\phi}_{m}, \phi_{m} \rangle \phi_{m}+\langle\Delta \phi_{m}, \hat{\phi}_{m}\rangle \Delta \phi_{m}) d t\\
=& \sum_{n}^{N} \int \sigma_{n} \phi_{n} \cdot x_{n}(\langle\phi_{n}, \hat{\phi}_{n}\rangle \phi_{n}+\langle\phi_{n}, \hat{\phi}_{n} \rangle \Delta \phi_{n})\\
+&\sum_{m \neq n}^{N} \sigma_{n} \phi_{n} \cdot x_{m}(\langle\phi_{m}, \hat{\phi}_{n}\rangle \phi_{m}+\langle\Delta \phi_{n}, \hat{\phi}_{m}\rangle \Delta \phi_{n}) d t\\
=& \sum_{n}^{N}\{\sigma_{n} x_{n}\langle \phi_{n} \hat{\phi}_{n}\rangle \cdot \int \phi_{n} \phi_{n} d t +\sigma_{n} x_{n}\langle\Delta \phi_{n}, \hat{\phi}_{n}\rangle \cdot\int \phi_{n} \Delta \phi_{n} d t \\
+&\sum_{m \neq n}^{N}[\sigma_{n} x_{m}\langle\phi_{m}, \hat{\phi}_{m}\rangle \cdot \int \phi_{n} \phi_{m} d t+\sigma_{n} x_{m}\langle \Delta \phi_{m} \hat{\phi}_{m} \rangle \int \Delta \phi_{m} \phi_{n} d t]\} \\
=& \sum_{n}^{N}[\sigma_{n} x_{n}\langle\phi_{n}, \hat{\phi}_{n}\rangle+\sum_{m}^{N} \sigma_{n} x_{m}\langle\Delta \phi_{m}, \hat{\phi}_{m}\rangle \int \phi_{n} \Delta \phi_{m} d t]\\
=& \sum_{n}^{N}[\sigma_{n} x_{n}\langle\phi_{n}, \hat{\phi}_{n}\rangle+\sum_{m}^{N} \sigma_{n} x_{m}\langle\Delta \phi_{m}, \hat{\phi}_{m}\rangle \langle \phi_{n}, \Delta \phi_{m} \rangle]\\
\end{aligned}
\end{equation}

We also have 

\begin{equation}
\begin{aligned}
E\{H \tilde{X}\} &=\int \sum_{n}^{N} \sigma_{n} \phi_{n}  \cdot \sum_{m}^{N} x_{m} \phi_{m} d t \\
&=\sum_{n} \sigma_{n} x_{n} .
\end{aligned}
\end{equation}

Thus the MSE caused by imperfect CSI is given by
\begin{equation}
\begin{aligned}
& E\{|\Delta H \tilde{X}|^{2}\}= E\{|H \Delta X|^{2}\} = E\{|H X-H \tilde{X}|^{2}\}\\
=&E\{| \sum _ { n } [ \sigma_{n} x_{n} ( \langle\phi_{n}, \hat{\phi}_{n}\rangle -1) +\sum_{m}^{N} \sigma_{n} x_{m}\langle\Delta \phi_{m}, \hat{\phi}_{m}\rangle \langle\Delta \phi_{m}, \phi_{n}\rangle ]|^{2} \} \\
=&E\{|\sum_{n}^{N} \sigma_{n}[x_{n}(\langle\phi_{n}, \hat{\phi}_{n}\rangle-1) +\sum_{m}^{N} x_{m}\langle\Delta \phi_{m}, \hat{\phi}_{m}\rangle\langle \Delta \phi_{m}, \phi_{n}\rangle]|^{2}\}\\
=& \sum_{n}^{N} E\{\sigma_{n}^{2}|x_{n}(\langle\phi_{n}, \hat{\phi}_{n}\rangle-1)+\sum_{m}^{N} x_{m}\langle\Delta \phi_{m}, \hat{\phi}_{m}\rangle\langle\Delta \phi_{m}, \phi_{n}\rangle|^{2}\} \\
&+\sum_{n^{'} \neq n}^{N} E\{\sigma_{n^{'}} \sigma_{n} \cdot |\cdots|^{2}\},
\end{aligned}
\end{equation}

where $|\cdots|^2$ is the residual part, which is uncorrelated with $\sigma_n$. 
Meanwhile $E \{ \sigma_n \sigma_{n^{'}} \} = 0$ for $n \neq n^{'}$ , so the last item is $0$. Then We have

\begin{equation}
\begin{aligned}
&E\{|\Delta H \tilde{X}|^{2}\}\\
=& \sum_{n}^{N} \sigma_{n}^{2} E\{|x_{n}(\langle\phi_{n}, \hat{\phi}_{n}\rangle-1)+\sum_{m}^{N} x_{m}\langle\Delta \phi_{m}, \hat{\phi}_{m}\rangle\langle\Delta \phi_{m}, \phi_n \rangle|^{2}\} \\
=& \sum_{n}^{N} \sigma_{n}^{2} E\{| x_{n}[(\langle\phi_{n}, \hat{\phi}_{n}\rangle-1) + \langle\Delta \phi_{m}, \hat{\phi}_{m}\rangle\langle\Delta \phi_{m}, \phi_{n}\rangle]\\
&+\sum_{m \neq n} x_{m}\langle\Delta \phi_{m}, \hat{\phi}_{m}\rangle\langle \Delta \phi_{m}, \phi_{n}\rangle|^{2}\}\\
=&\sum_{n}^{N} \sigma_{n}^{2} E\{ x_{n}^{2}[(\langle\phi_{n}, \hat{\phi}_{n}\rangle-1)+ \langle\Delta \phi_{m}, \hat{\phi}_{m}\rangle\langle\Delta \phi_{m}, \phi_{n} \rangle]^{2}\\
&+\sum_{m \neq n}^{N} x_{m}^{2}(\langle\Delta \phi_{m}, \hat{\phi}_{m}\rangle\langle\Delta \phi_{m}, \phi_{n} \rangle)^{2}\} + \sum_{n^{'} \neq n}E \{x_{n^{'}} x_{n} \cdot |\cdots|^{2}\}.
\end{aligned}
\end{equation}

Also, $|\cdots|$ is uncorrelated with $x_n$ and $E \{ x_n x_{n^{'}} \} = 0$ for $n \neq n^{'}$. So, we have
\begin{equation}
\begin{aligned}
&E\{|\Delta H \tilde{X}|^{2}\}\\
=&\sum_{n}^{N} \sigma_{n}^{2} \{ x_{n}^{2}[(\langle\phi_{n}, \hat{\phi}_{n}\rangle-1) + \langle\Delta \phi_{m}, \hat{\phi}_{m}\rangle \langle\Delta \phi_{m}, \phi_{n} \rangle]^{2}\\
&+\sum_{m \neq n}^{N} x_{m}^{2}\langle\Delta \phi_{m}, \hat{\phi}_{m}\rangle ^2 \langle\Delta \phi_{m}, \phi_{n} \rangle^{2}\}.
\end{aligned}
\end{equation}

% \note{The objective function can choose minimizing MSE $E\{|\Delta H \tilde{X}|^{2}\}$ or maximizing the SINR}

% \begin{equation}
% \argmax_{\{x_{n}\} \{\hat{\phi}_{n}\}} \mathrm{SINR}=\frac{E\{|H \tilde{X}|^2\}}{\sigma_W^{2}+E\{|\Delta H \tilde{X}|^2\}}
% \end{equation}

% \begin{equation}
% E\{||H X||^2\} = \iiiint \mathcal{C}_{\mathbf{H}}(t, f ; \tau, \nu) \cdot \sigma^2 |\phi|^2 \mathrm{d} t \mathrm{d} f \mathrm{d} \tau \mathrm{d} \nu
% \end{equation}

\section{Proof of Corollary~\ref{corollary_1}}
\label{app:corollary_1}
The expected capacity of SISO channel $H(t)$ can be obtained by
\begin{equation}
\begin{aligned}
\bar{C}&=\max E\left\{\log _{2} \operatorname{det}\left(I+\frac{H(t) Q(t) H(t)}{I \cdot \sigma_{z}^{2}}\right)\right\}\\
&=\max \log _{2} \operatorname{det}\left(I+\frac{E\{H(t) Q(t) H(t)\}}{I \cdot \sigma_{z}^{2}}\right)\\
&\text { s.t. } E\{\operatorname{tr}(Q(t))\} \leqslant P
\end{aligned}
\end{equation}

Assume the channel $H(t)$ is completely known and is decomposed by KLT $H = \sum_{n=1}^ \infty \sigma_n \phi_n(t)$. Then we have

\begin{equation}
\begin{aligned}
&E\{H(t)Q(t)H^H(t)\}\\
=&E\{\sum_{n=1}^ \infty \sigma_n \phi_n(t) Q(t) \sum_{m=1}^ \infty \sigma_m \phi_m^H(t)\}\\
=&E\{\sum_{n=1}^ \infty \sigma_n^2 \phi_n(t) Q(t) \phi_n^H(t) + \sum_{m\neq n}^ \infty \sigma_n \sigma_m \phi_n(t) Q(t) \phi_m^H(t)\}\\
=&E\{\sum_{n=1}^ \infty \sigma_n^2 \phi_n(t) Q(t) \phi_n^H(t)\} + \sum_{m\neq n}^ \infty E\{\sigma_n \sigma_m\} E\{\phi_n(t) Q(t) \phi_m^H(t)\}\\
\end{aligned}
\end{equation}

Because $E\{\sigma_n \sigma_m\} = 0 $ for $m\neq n$, the second item is 0. Let $X(t) = \sum_{n=1}^ \infty x_n \phi_n(t)$, where $x_n = \int X(t) \phi_n(t) dt$. Then we have 
\begin{equation}
\begin{aligned}
& E\{H(t)Q(t)H^H(t)\}=E\{\sum_{n=1}^ \infty \sigma_n^2 \phi_n(t) Q(t) \phi_n^H(t)\} \\
=&\sum_{n=1}^ \infty \sigma_n^2 \int \phi_n(t) Q(t) \phi_n^H(t) dt\\
=&\sum_{n=1}^ \infty \sigma_n^2 \int \phi_n(t) \sum_{l=1}^ \infty x_l \phi_l(t) \sum_{m=1}^ \infty x_m \phi_m^H(t) \phi_n^H(t) dt\\
=&\sum_{n=1}^ \infty \sigma_n^2 x_n^2\int \phi_n(t) \phi_n(t) \phi_n^H(t) \phi_n^H(t) dt\\
=&\sum_{n=1}^ \infty \sigma_n^2 x_n^2 \cdot I
\end{aligned}
\end{equation}

One the other hand,
\begin{equation}
\begin{aligned}
E\{\operatorname{tr}(Q(t))\} &= \operatorname{tr}(E[\sum_{n=1}^ \infty x_n \phi_n(t) \sum_{m=1}^ \infty x_m \phi_m^H(t)])\\
&=\operatorname{tr}(\sum_{n=1}^ \infty x_n^2\int \phi_n(t) \phi_n(t) \phi_n^H(t) \phi_n^H(t) dt)\\
&=\operatorname{tr}(\sum_{n=1}^ \infty x_n^2 \cdot I)\\
&=\sum_{n=1}^ \infty x_n^2 \leqslant P
\end{aligned}
\end{equation}

Hence, 
\begin{equation}
\begin{aligned}
\bar{C}&=\argmax_{(\sum_{n=1}^ \infty x_n^2) \leqslant P} \log _{2} \operatorname{det}\left(I+\frac{\sum_{n=1}^ \infty \sigma_n^2 x_n^2 \cdot I}{I \cdot \sigma_{z}^{2}}\right)\\
&=\argmax_{(\sum_{n=1}^ \infty x_n^2) \leqslant P} \sum_{n=1}^ \infty \log _{2} \left(1+\frac{ \sigma_n^2 x_n^2 }{\sigma_{z}^{2}}\right)\\
\end{aligned}
\end{equation}

Using WF algorithm, the optimal solution is 
\begin{equation}
    x_n^2 = \left(\mu - \frac{\sigma_z^2}{\sigma_n^2}\right)^{+}
\end{equation}
where $\mu$ is a constant and $(x)^{+}$ is defined as
\begin{equation}
(x)^{+}=\left\{\begin{array}{ll}
x & \text { if } x \geq 0 \\
0 & \text { if } x<0
\end{array}\right.
\end{equation}

Which is the same with SVD precoding.
\end{comment}
